# Supplementary material for: Secure Arithmetic Computation with No Honest Majority
Source: arXiv:0811.0475 source file (2008-11-08)
Supplement: Supplementary file 1 [file appendix.tex]

\section{Proof of Lemma~\ref{lem:adaptive}}
\label{app:pf-adaptive}
